# Supplementary material for: Clustering with missing data: which imputation model for which cluster analysis method?
Source: arXiv:2106.04424 source file (2021-06-08)
Supplement: Supplementary file 1 [file wineappendix.tex]

\subsection*{Wine data set}
\subsubsection*{MCAR}
\begin{table}[H]
\centering
\small
\caption{\label{varselwine}Conditional models for FCS MI under a MCAR mechanism: matrix specifying the set of predictors used for each variable to be imputed. Each row corresponds to a variable to be imputed. A value of 1 means that the column variable is used as a predictor for the target in the rows.}
\begin{tabular}{rrrrrrrrrrrrrr}
  \hline
 & \begin{sideways} Alcohol \end{sideways} & \begin{sideways} Malic acid \end{sideways} & \begin{sideways} Ash \end{sideways} & \begin{sideways} Alcalinity of ash \end{sideways} & \begin{sideways} Magnesium \end{sideways} & \begin{sideways} Total phenols \end{sideways} & \begin{sideways} Flavanoids \end{sideways} & \begin{sideways} Nonflavanoid phenols \end{sideways} & \begin{sideways} Proanthocyanins \end{sideways} & \begin{sideways} Color intensity \end{sideways} & \begin{sideways} Hue \end{sideways} & \begin{sideways} OD280/OD315 of diluted wines \end{sideways} & \begin{sideways} Proline \end{sideways} \\ 

  \hline
Alcohol & 0 & 1 & 0 & 1 & 0 & 0 & 1 & 0 & 0 & 1 & 1 & 0 & 1 \\ 
  Malic acid & 1 & 0 & 1 & 1 & 0 & 1 & 1 & 1 & 1 & 0 & 1 & 1 & 0 \\ 
  Ash & 1 & 1 & 0 & 1 & 1 & 1 & 1 & 1 & 0 & 1 & 1 & 0 & 1 \\ 
  Alcalinity of ash & 1 & 1 & 1 & 0 & 0 & 0 & 1 & 0 & 0 & 1 & 1 & 0 & 1 \\ 
  Magnesium & 0 & 0 & 0 & 1 & 0 & 0 & 1 & 1 & 1 & 1 & 0 & 0 & 1 \\ 
  Total phenols & 1 & 0 & 0 & 0 & 1 & 0 & 1 & 0 & 1 & 1 & 0 & 1 & 1 \\ 
  Flavanoids & 1 & 1 & 1 & 1 & 1 & 1 & 0 & 1 & 1 & 1 & 1 & 1 & 1 \\ 
  Nonflavanoid phenols & 1 & 1 & 0 & 0 & 0 & 1 & 1 & 0 & 0 & 0 & 1 & 0 & 0 \\ 
  Proanthocyanins & 0 & 0 & 0 & 1 & 1 & 1 & 0 & 1 & 0 & 0 & 0 & 1 & 0 \\ 
  Color intensity & 0 & 0 & 1 & 0 & 1 & 1 & 1 & 0 & 1 & 0 & 1 & 1 & 1 \\ 
  Hue & 1 & 1 & 1 & 0 & 0 & 0 & 1 & 1 & 1 & 1 & 0 & 1 & 1 \\ 
  OD280/OD315 of diluted wines & 1 & 0 & 0 & 0 & 1 & 1 & 0 & 0 & 1 & 1 & 1 & 0 & 1 \\ 
  Proline & 0 & 0 & 1 & 0 & 1 & 0 & 0 & 0 & 1 & 1 & 0 & 1 & 0 \\ 
   \hline
\end{tabular}
\end{table}

\begin{table}[H]
\centering
\small
\caption{Number of clusters for wine data set under a MCAR mechanism: total instability according to the number of clusters $\Nbgroup$ for various MI methods and various cluster analyses. A suitable number of clusters can be obtained by identifying a ``kick'' across the set of instability values. \label{nbgroupwine}} 
\begin{tabular}{llrrrrr}
  \hline
clustering & MI & $\Nbgroup= 2$ & $\Nbgroup= 3$ & $\Nbgroup= 4$ & $\Nbgroup= 5$ & $\Nbgroup= 6$ \\ 
  \hline
%mixture & FCS-norm & 0.43 & 0.46 & 0.42 & 0.38 & 0.34 \\ 
%  pam & FCS-norm & 0.28 & 0.31 & 0.34 & 0.31 & 0.29 \\ 
%  hc & FCS-norm & 0.32 & 0.35 & 0.33 & 0.30 & 0.29 \\ 
%  kmeans & FCS-norm & 0.23 & 0.19 & 0.25 & 0.26 & 0.25 \\ 
   pam & JM-GL & 0.20 & 0.15 & 0.22 & 0.25 &  \\ 
  hc & JM-GL & 0.11 & 0.14 & 0.18 & 0.20 &  \\ 
  kmeans & JM-GL & 0.13 & 0.09 & 0.16 & 0.18 &  \\ 
%  mixture & JM-DP & 0.54 & 0.49 & 0.45 & 0.39 & 0.35 \\ 
%  pam & JM-DP & 0.33 & 0.34 & 0.35 & 0.33 & 0.31 \\ 
%  hc & JM-DP & 0.45 & 0.36 & 0.34 & 0.32 & 0.30 \\ 
%  kmeans & JM-DP & 0.28 & 0.23 & 0.28 & 0.28 & 0.27 \\ 
  mixture & FCS-hetero & 0.43 & 0.35 &  &  &  \\ 
  pam & FCS-hetero & 0.36 & 0.26 &  &  &  \\ 
  hc & FCS-hetero & 0.38 & 0.24 &  &  &  \\ 
  kmeans & FCS-hetero & 0.28 & 0.16 &  &  &  \\ 
  mixture & FCS-homo & 0.39 & 0.26 & 0.26 & 0.29 & 0.27 \\ 
  pam & FCS-homo & 0.24 & 0.22 & 0.25 & 0.27 & 0.25 \\ 
  hc & FCS-homo & 0.27 & 0.21 & 0.22 & 0.23 & 0.22 \\ 
  kmeans & FCS-homo & 0.22 & 0.13 & 0.19 & 0.20 & 0.20 \\ 
   \hline
\end{tabular}
\end{table}
\subsubsection*{MAR}

\begin{table}[H]
\centering
\small
\caption{\label{varselwine_mar}Conditional models for FCS MI under a MAR mechanism: matrix specifying the set of predictors used for each variable to be imputed. Each row corresponds to a variable to be imputed. A value of 1 means that the column variable is used as a predictor for the target in the rows.}
\begin{tabular}{rrrrrrrrrrrrrr}
  \hline
 & \begin{sideways} Alcohol \end{sideways} & \begin{sideways} Malic acid \end{sideways} & \begin{sideways} Ash \end{sideways} & \begin{sideways} Alcalinity of ash \end{sideways} & \begin{sideways} Magnesium \end{sideways} & \begin{sideways} Total phenols \end{sideways} & \begin{sideways} Flavanoids \end{sideways} & \begin{sideways} Nonflavanoid phenols \end{sideways} & \begin{sideways} Proanthocyanins \end{sideways} & \begin{sideways} Color intensity \end{sideways} & \begin{sideways} Hue \end{sideways} & \begin{sideways} OD280/OD315 of diluted wines \end{sideways} & \begin{sideways} Proline \end{sideways} \\ 

  \hline
Alcohol & 0 & 1 & 0 & 1 & 1 & 1 & 0 & 0 & 1 & 1 & 1 & 1 & 1 \\ 
  Malic acid & 1 & 0 & 1 & 0 & 0 & 0 & 1 & 1 & 0 & 1 & 1 & 1 & 0 \\ 
  Ash & 1 & 1 & 0 & 1 & 1 & 1 & 1 & 1 & 1 & 1 & 0 & 0 & 1 \\ 
  Alcalinity of ash & 1 & 1 & 1 & 0 & 0 & 1 & 1 & 1 & 1 & 1 & 1 & 0 & 1 \\ 
  Magnesium & 1 & 1 & 0 & 1 & 0 & 0 & 0 & 1 & 1 & 1 & 0 & 0 & 0 \\ 
  Total phenols & 1 & 1 & 1 & 0 & 1 & 0 & 1 & 1 & 1 & 0 & 1 & 1 & 1 \\ 
  Flavanoids & 1 & 0 & 1 & 0 & 1 & 1 & 0 & 1 & 1 & 1 & 1 & 1 & 1 \\ 
  Nonflavanoid phenols & 1 & 1 & 1 & 1 & 0 & 1 & 1 & 0 & 1 & 1 & 1 & 1 & 1 \\ 
  Proanthocyanins & 1 & 0 & 0 & 0 & 1 & 1 & 1 & 1 & 0 & 0 & 0 & 1 & 1 \\ 
  Color intensity & 1 & 1 & 1 & 1 & 0 & 0 & 0 & 1 & 1 & 0 & 1 & 1 & 1 \\ 
  Hue & 1 & 0 & 0 & 0 & 0 & 1 & 1 & 0 & 1 & 1 & 0 & 1 & 0 \\ 
  OD280/OD315 of diluted wines & 1 & 1 & 0 & 0 & 1 & 1 & 1 & 1 & 1 & 1 & 1 & 0 & 1 \\ 
  Proline & 1 & 1 & 1 & 1 & 1 & 1 & 1 & 1 & 1 & 0 & 1 & 1 & 0 \\ 
   \hline
\end{tabular}
\end{table}

\begin{table}[H]
\centering
\small
\caption{Number of clusters for wine data set under a MAR mechanism: total instability according to the number of clusters $\Nbgroup$ for various MI methods and various cluster analyses. A suitable number of clusters can be obtained by identifying a ``kick'' across the set of instability values. \label{nbgroupwine_mar}} 
\begin{tabular}{llrrrrr}
  \hline
clustering & MI & $\Nbgroup= 2$ & $\Nbgroup= 3$ & $\Nbgroup= 4$ & $\Nbgroup= 5$ & $\Nbgroup= 6$ \\ 
  \hline
mixture & JM-GL & 0.23 & 0.20 & 0.19 & 0.25 & 0.23 \\ 
  pam & JM-GL & 0.32 & 0.18 & 0.23 & 0.24 & 0.25 \\ 
  hc & JM-GL & 0.37 & 0.17 & 0.17 & 0.22 & 0.23 \\ 
  kmeans & JM-GL & 0.25 & 0.09 & 0.13 & 0.21 & 0.20 \\ 
  mixture & FCS-hetero & 0.26 & 0.28 &  &  &  \\ 
  pam & FCS-hetero & 0.37 & 0.22 &  &  &  \\ 
  hc & FCS-hetero & 0.26 & 0.24 &  &  &  \\ 
  kmeans & FCS-hetero & 0.18 & 0.13 &  &  &  \\ 
  mixture & FCS-homo & 0.43 & 0.24 & 0.23 & 0.26 & 0.27 \\ 
  pam & FCS-homo & 0.24 & 0.18 & 0.25 & 0.25 & 0.24 \\ 
  hc & FCS-homo & 0.34 & 0.18 & 0.18 & 0.21 & 0.22 \\ 
  kmeans & FCS-homo & 0.21 & 0.11 & 0.14 & 0.18 & 0.20 \\ 
   \hline
\end{tabular}
\end{table}
