# Supplementary material for: Clustering with missing data: which imputation model for which cluster analysis method?
Source: arXiv:2106.04424 source file (2021-06-08)
Supplement: Supplementary file 2 [file frogicuappendix.tex]

\subsection*{FROG-ICU study}
